# Supplementary material for: Non-Hermitian Hamiltonians for Linear and Nonlinear Optical Response: a Model for Plexcitons
Source: arXiv:2206.13265 source file (2023-05-08)

Weak coupling

Strong coupling

Point D

Point E

Point F

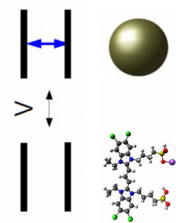 $\mu_j=0$ 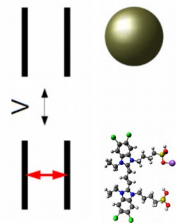 $\mu_p=0$ 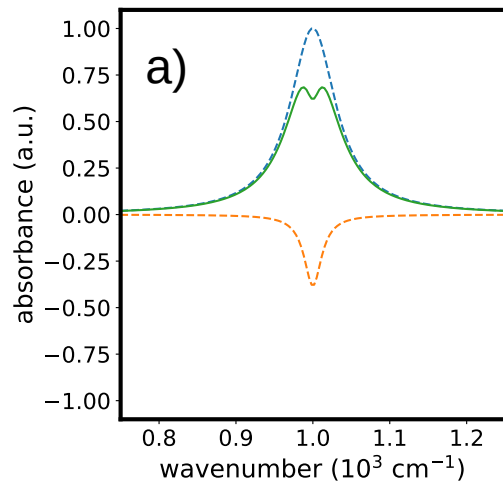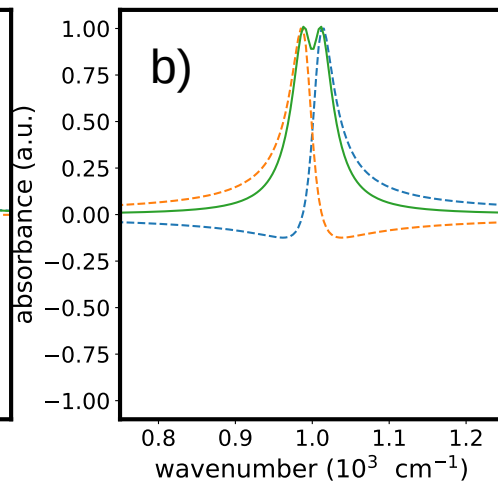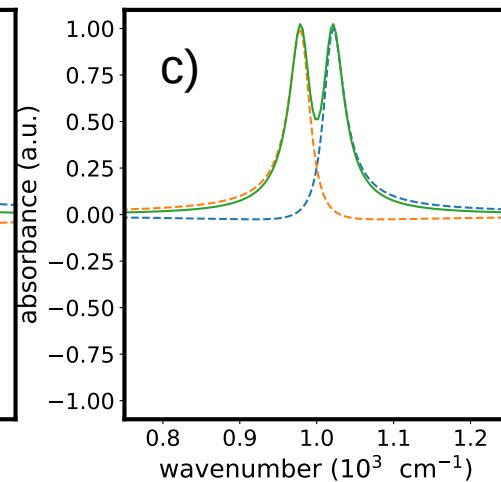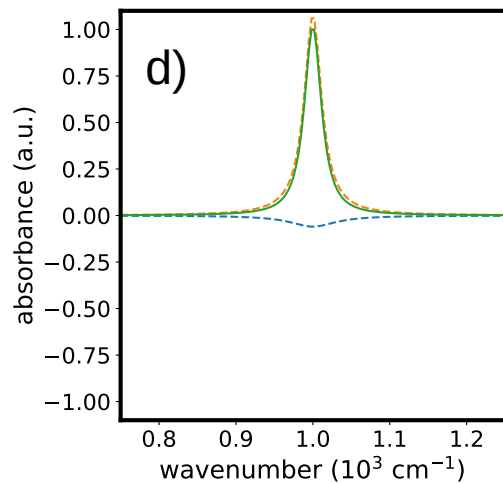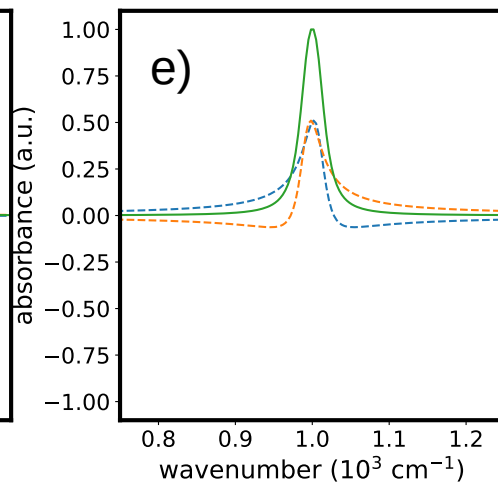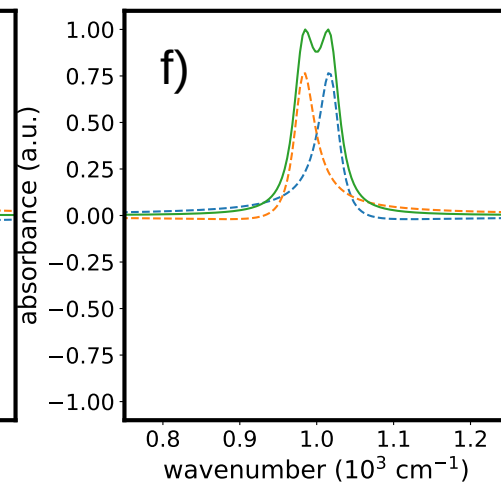

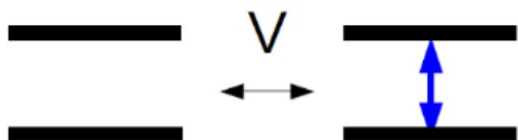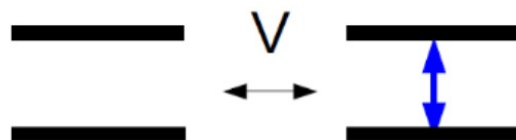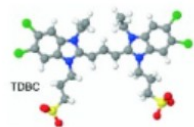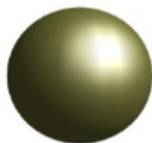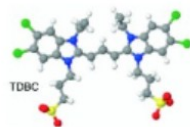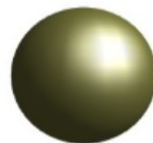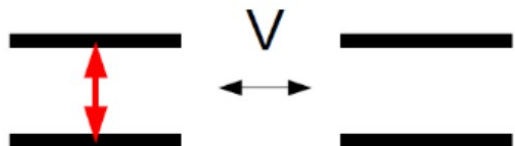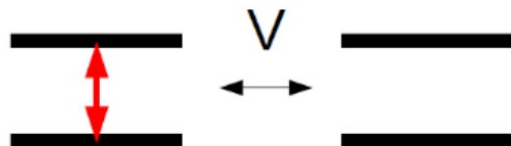

Supplement: Supplementary file 1 [file Figure_SI_other_points.pdf]
